# Supplementary material for: Accurate Uncertainty Estimation and Decomposition in Ensemble Learning
Source: arXiv:1911.04061 source file (2019-11-11)
Supplement: Supplementary file 1 [file appendix.tex]

\section{Prior Specification for $G$: Constrained Gaussian Process}
\label{sec:cgp}

Assuming modeling $G \sim GP(0, k(\bz, \bz'))$ with the data pair $\{y, \bz\}$ and denote $g = \frac{\partial}{\partial \bz} G$ the derivative of $G$, a \textit{constrained Gaussian process}  \citep{riihimaki_gaussian_2010, lorenzi_constraining_2018, liu_gaussian_2019} imposes the monotonicity  constraint $\Csc = \{G| g \geq 0 \}$ and boundedness constraint $\Csc=\{G | G \geq 0, 1 - G \geq 0\}$ onto $G$ by explicitly modeling the joint posterior $f(G, g | y, \bz, \Csc)$ as:
\begin{align}
P(G, g|\Csc, y, \bz) \propto
P(y| G, \bz)
P(\Csc|G, g)
P(G, g).
\label{eq:mono_gp}
\end{align}
Here $P(y|G, \bz)$ is the likelihood function for $y|G(\bz)$. $P(\Csc | g )$ is the likelihood for the non-negativity constraint $\Csc$ that assigns near zero probability to the $G$'s that have negative derivative or take value outside $[0, 1]$. In this work, we consider $P(\Csc |G, g) \propto \Phi_\sigma \big( g \big) * \Phi_\sigma \big( G \big) * \Phi_\sigma \big( 1 - G \big)$ where $\Phi_\sigma$ denotes the Gaussian CDF with variance $\sigma$. The variance parameter of $\Phi$ can be adjusted to specify the strength of regularization \citep{lorenzi_constraining_2018}, which we set to $\sigma=0.01$ so $P(\Csc |G, g)$ drops quickly to zero in regions outside the feasibility constraint.
Finally, $P(G, g)$ is the joint prior for the Gaussian process $G$ and its derivative $g$. Specifically, since differentiation is a linear operator, for $G(\bz) \sim GP(0, k(\bz, \bz'))$, the derivative $g(\bz) \sim GP(0, \deriv{\bz \partial \bz'}k(\bz, \bz'))$ is again a Gaussian process. Therefore, conditional on $\bz$, $(G, g)$ is jointly multivariate Gaussian and the $P(G, g)$ takes the form \citep{rasmussen_gaussian_2006}:
\begin{align*}
\begin{bmatrix}
G(\bz) \\ g(\bz)
\end{bmatrix} \sim 
\phi \Bigg(
\begin{bmatrix} 0 \\ 0 \end{bmatrix}, 
\begin{bmatrix} 
k(\bz, \bz') & \partial_{\bz'} k(\bz, \bz') \\
\partial_{\bz} k(\bz, \bz') & \partial_{\bz}\partial_{\bz'} k(\bz, \bz')
\\\end{bmatrix}
\Bigg).
\end{align*}
Similar to \gls{GP}, the \gls{CGP} prior is proper and comes with a theoretical guarantee in posterior convergence for a wide range of learning settings \citep{liu_gaussian_2019, van_der_vaart_rates_2008}.

\section{Posterior Inference}
\label{sec:inference}

\subsection{Posterior Likelihood}
To ensure efficient posterior sampling, we integrate out $G$ and $\delta$ from the model posterior, and express the model compactly as $F^*(y|\bx) = F(y|\bx, \mu)$ with prior:
\begin{align}
     \quad
    F | \mu \sim CGP\big( \Phi_\epsilon(y|\bx, \mu), k_G \big), \quad
    \mu | \omega \sim GP\big( \sum_k f_k(\bx) \omega_k, k_\mu \big),
\label{eq:compact_bne_model}
\end{align}
and to avoid parameter non-identifiability, we orthogonalize $k_G$ and $k_\mu$ with respect to their mean functions $\Phi_\epsilon$ and $\sum_k f_k(\bx)$ \citep{reich_effects_2006, maceachern_comment_2007}. Specifically, given a kernel matrix $\bK$ generated by the kernel function $k$, and a mean function matrix $\bF_{N \times K}$ that corresponds to the $K$ mean functions evaluated at $N$ data points, we can compute the orthogonal projection matrix to the residual space of mean function as $\bP_{N \times N} = \bI - \bF(\bF^\top\bF)^{-1}\bF^\top$ where $\bF_{N \times K}$, and compute the orthogonalized kernel matrix as $\bK = \bP\bK\bP^\top$ \citep{reich_effects_2006}.

Consequently, given observations $\Dsc=\{y_i, \bx_i\}_{i=1}^N$, denoting 
%$\Phi$ the standard Gaussian \gls{CDF} and 
$\phi(.|\bm, \bS)$ the Gaussian \gls{PDF} with mean $\bm$ and covariance function $\bS$, \gls{BNE}'s model posterior $p_{\Dsc}$ is a simple product of model \gls{PDF}s $f = \deriv{y} F$ and Gaussian distribution functions:
\begin{align}
    p_{\Dsc}(F, \mu) 
    &\propto 
    \Big[\prod_{i=1}^N f(y_i|\bx_i, \mu) \Big] * 
    p\big(f\big|\mu \big) * p\big(\mu\big|\omega \big) * p\big(\omega\big),
    \label{eq:bne_posterior}
    % \\
    % &\propto 
    % \Big[\prod_{i=1}^N f(y_i|\bx_i, \mu) \Big] * 
    % \Big[\phi \big( f \big| \phi(y_i|\bx_i, \mu), \bK_G \big)\Big] * 
    % \phi \Big( \mu | \sum_k f_k \omega_k, \bK_\mu \Big) * 
    % \phi \Big( \bomega | 0, \sigma^2_\omega \bI \Big)
\end{align}
where $p(\mu \big| \omega)$ is the standard \gls{GP} likelihood, and $p(\omega)$ is the zero-mean Gaussian likelihood $N(0, \sigma_\omega^2\bI)$, and $p\big(f\big|\mu \big)$ is the \gls{CGP} likelihood specified in (\ref{eq:mono_gp}), i.e.:
\begin{align}
    p(f|\mu) = 
    \phi \Big(
    F, f \Big| 
    \begin{bmatrix} \Phi_\epsilon(.|\mu) \\ \phi_\epsilon(.|\mu) \end{bmatrix},
    \begin{bmatrix} 
            k & \partial_{\bz'} k \\
            \partial_{\bz} k & \partial_{\bz}\partial_{\bz'} k
    \end{bmatrix}
    \Big)
    *
    \Phi_\sigma(F)\Phi_\sigma(1-F)\Phi_\sigma(f),
\end{align}
where $\Phi_\epsilon$ and $\phi_\epsilon$ are the model \gls{CDF} and \gls{PDF} of the $\delta$-agumented ensemble (\ref{eq:model_system}).

\subsection{Hyperparameters}
\label{sec:hyper}

\gls{BNE}'s hyper-parameters are the Mat\'{e}rn length-scale parameters $l_\delta$ and $l_G$, and the prior variances $\sigma_\omega$ and $\sigma_\epsilon$. Consistent with the existing \gls{GP} approaches, we place the inverse-Gamma priors on the $l_\delta$ and $l_G$ and the Half Normal priors on $\sigma_\omega$ and $\sigma_\epsilon$ \citep{team_stan_nodate}, i.e.:
\begin{align*}
l_\delta &\sim invGamma(\alpha_\delta, \beta_\delta)
\quad
l_G  \sim invGamma(\alpha_G, \beta_G)
\end{align*}
where $\alpha$, $\beta$ where chosen so the prior probability for $l$ falling into a desired range $[l_{lower}, l_{upper}]$ is high. In this work, we set $l_{lower}=2$ and $l_{upper}=10$ such that $P_{invGamma}(l \in [2, 10]|\alpha, \beta)=0.98$ for both $l_\delta$ and $l_G$.  Finally, we use the weakly informative half-Gaussian priors for the variance parameters:
\begin{align*}
\sigma_\omega &\sim HalfNormal(0, 5)
\quad
\sigma_\epsilon \sim HalfNormal(0, 5)
\end{align*}

\subsection{Computation}

To fully capture the model uncertainty encoded in the posterior distribution, 
We perform posterior inference using \gls{HMC} \citep{neal_mcmc_2012}, and we use the adaptive step size proposed in \citep{andrieu_tutorial_2008} with implementation available in TensorFlow Probability \citep{dillon_tensorflow_2017}. Given data $\Dsc$ of size $N$, we first estimate the value of the hyper-parameters $\{l_\delta, l_G, \sigma_\omega, \sigma_\epsilon\}$ through an empirical Bayes approach by maximizing the posterior likelihood regularized by the hyper-parameter priors specified in \ref{sec:hyper}. We then perform full MCMC with respect to the posterior likelihood (\ref{eq:bne_posterior}), fixing the hyperparamters to their estimated values from the empirical Bayes procedure.

The computation complexity of sampling from \gls{BNE} posterior is $O(N^3)$ due to the need of inverting \gls{GP} kernel matrices. In the case of very large datasets, we consider the simple parallel MCMC scheme proposed in \cite{li_simple_2017} which is dedicated to estimating posterior quantiles (i.e. the inverse \gls{CDF}s). This method divides the dataset into $K$ subsets and run MCMC with respect to an adjusted posterior in parallel in each subset. As a result the computation complexity is reduced to $O(N^3/K^3)$ in the case of $K$ machines, or $O(N^3/K^2)$ in the case of a single machine.

\section{Posterior Consistency of BNE}
\label{sec:bne_consistency_proof}
\begin{proof}
Analogous to Theorem 3.2 of \cite{van_der_vaart_rates_2008}, we show Theorem \ref{thm:bne_consistency} by invoking Theorem 2.1 of \cite{ghosal_convergence_2000} which shows the posterior consistency for general Bayesian models, provided that  certain conditions on the model likelihood and the prior distribution are satisfied (i.e. condition (\ref{eq:conv_cond_orig_3})-(\ref{eq:conv_cond_orig_1}) in below theorem). For completeness, we state the theorem below:

\begin{theorem_app}[Posterior Consistency for General Bayesian Models]
Let $\{y_i, \bx_i\}_{i=1}^n \sim P^*(y|\bx)$, and let $P \sim \Pi_n$ be a sequence of prior probability with support on $B$, and $||.||$ a metric on $B$. Denote $N(\epsilon, B, d)$ the $\epsilon$-packing number for set $B$ with respect to metric $||.||$, also denote $KL(P, P^*)$ the \gls{KL} divergence, and $V(P, P^*)=E^*\big(log(\frac{P}{P^*})^2\big)$ the $L_2$ metric for log likelihood ratio between $P$ and $P^*$.

Suppose that for a sequence $\epsilon_n \rightarrow 0$ and $n \epsilon_n^2 \rightarrow \infty$, a constant $C$ and a sequence of set $B_n$, we have:
\begin{align}
    log \, N(\epsilon_n, B_n, ||.||) 
    &\leq n\epsilon_n^2 
    \tag{\ref{thm:post_conv}-I}
    \label{eq:conv_cond_orig_3} \\
    \Pi_n(B \backslash B_n) 
    &\leq exp(-n\epsilon^2_n(C+4))
    \tag{\ref{thm:post_conv}-II}
    \label{eq:conv_cond_orig_2} \\
    \Pi_n \Big( KL(P, P^*) \vee V(P, P^*) \leq \epsilon_n^2 \Big)
    &\geq exp(-n \epsilon_n^2 C)
    \tag{\ref{thm:post_conv}-III}
    \label{eq:conv_cond_orig_1} 
\end{align}
Then for sufficiently large $M$, we have that in probability:
\begin{align*}
    \Pi_n \Big( d(P, P_0) \geq M \epsilon_n \Big| \{y_i, \bx_i\}_{i=1}^n \Big) \rightarrow 0
\end{align*}
\label{thm:post_conv}
\end{theorem_app}
Therefore to show posterior consistency, only need to show the three conditions in above theorem hold. To this end, we make use of the below theorem from \cite{liu_gaussian_2019} which derives the aforementioned conditions for \gls{CGP}. We state this theorem below:
\begin{theorem_app}[Conditions for Posterior Consistency in \gls{CGP}]
Let $g$ be a Borel measurable, zero-mean constratined Gaussian random element in a separable Banach space $(\Bbb, ||.||_\infty)$ with \gls{RKHS} $(\Hsc_k, ||.||_{\Hsc_k})$. Define the concentration function $\psi_{g^*}(\epsilon) = \inf_{\hat{g} \in \Hsc_k, ||\hat{g} - g^*||_\infty \leq \epsilon} ||\hat{g}||^2_{\Hsc_k} - log \, P(||g||_\infty \leq \epsilon)$. 

For any number $\epsilon_n > 0$ satisfying $\psi_{g^*}(\epsilon_n) \leq n\epsilon_n^2$, and any constant $C \geq 1$ with $e^{-Cn\epsilon_n^2} < \frac{1}{2}*  \frac{E(f(\Csc|g))}{E(||g||_{\Hsc_k}^2)\vee 1}$, for $g^*$ a function contained in the closure of $\Hsc_k$ in $\Bbb$ that is $\epsilon_n$-feasible, there exists a measurable set $B_n \subset \Bbb$ such that:
\begin{align}
log \, N(2 \epsilon_n, B_n, ||.||) &\leq 2 C n \epsilon_n^2 
    \tag{\ref{thm:cgp_conv}-I}
\label{eq:conv_cond_3} \\
P(g \not\in B_n) &\leq e^{-Cn\epsilon_n^2} 
    \tag{\ref{thm:cgp_conv}-II}
\label{eq:conv_cond_2} \\
P(||g - g^*|| < 2\epsilon_n) &\geq e^{-n\epsilon_n^2} 
    \tag{\ref{thm:cgp_conv}-III}
\label{eq:conv_cond_1} 
\end{align}
\label{thm:cgp_conv}
\end{theorem_app}
%This is a result that is analogous to Theorem 2.1 in \cite{van_der_vaart_rates_2008} but designed for the constrained Gaussian process. Similar to \cite{van_der_vaart_rates_2008}, there exists a slight mismatch between  conditions (\ref{eq:conv_cond_3}) and (\ref{eq:conv_cond_orig_3}) in terms of an additional multiplicative constant $2C$, which, as commented by the original author, is of no substantive importance since we are only interested in rates of convergence.
Consequently, to show the posterior consistency for \gls{BNE} with respect to the $L_2$ metric $E^*\big(||F - F^*||_2\big)$, we only need to show the three conditions in Theorem \ref{thm:post_conv} is satisfied by making use of Theorem \ref{thm:cgp_conv}. 

Notice for sufficiently small $\epsilon_n$, $F^*$ is $\epsilon_n$-feasible (i.e. $E(f(\Csc|F^* + s)) > E(f(\Csc|s))$ where $s$ is a bounded random noise $s \sim GP(0, k)$ and $||s|| < \epsilon_n$, see \cite{liu_gaussian_2019} for full definition) since the zero function $\bzero(x)=0$ lies on the boundary of the constrain set $\Csc$, therefore we can apply Theorem \ref{thm:cgp_conv} for \gls{BNE}. Only left to check if the three conditions in Theorem \ref{thm:post_conv} are satisfied by making use of Theorem \ref{thm:cgp_conv}. It is easy to see that conditions \ref{eq:conv_cond_orig_3} and \ref{eq:conv_cond_orig_2} are satisfied by \ref{eq:conv_cond_3} and \ref{eq:conv_cond_2}. Therefore only need to show that condition \ref{eq:conv_cond_orig_1} also holds. To this end, notice that  by Lemma 3.2 of \cite{van_der_vaart_rates_2008} the $KL(P, P^*)$ and $V(P, P^*)$ metrics in condition (\ref{eq:conv_cond_orig_1}) is upper bounded by the $L_2$ metric (denoted as $||.||$) in equation (\ref{eq:conv_cond_1}) up to a multiplicative constant. Therefore \ref{eq:conv_cond_1} implies \ref{eq:conv_cond_orig_1}. As a result, the three conditions in Theorem \ref{thm:post_conv} are satisfied, which implies posterior convergence.
\end{proof}

\section{BNE's Predictive Distribution}
\label{sec:unc_decomp_deriv}

\paragraph{Expression for Model Predictive Mean}

Recall the ``Darth Vadar rule" \citep{muldowney_darth_2012}:
\begin{align}
E(s(y)|\bx) &= \int_{y \in \Ysc} 
\deriv{y}s(y) * \big[ I(y>0) - F(y|\bx) \big] dy
\label{eq:darth}
\end{align}
Also recall that \gls{BNE}'s model \gls{CDF} is $F(y|\bx, G, \Phi) = G \Big[ F_S(y|\bx, \Phi) \Big]$. Therefore we can expresse the predictive mean $E(y|\bx, G, \Phi)$ for full \gls{BNE} in terms of its CDF:
\begin{align*}
E(y|\bx, G, \Phi)
&= \int_{y \in \Ysc} I(y>0) - F(y|\bx, G, \Phi) dy\\
&= \int_{y \in \Ysc} I(y>0) - G \Big[ F_S(y|\bx, \Phi) \Big] dy \\
&= \int_{y \in \Ysc} 
\Big[ I(y>0) - F_S(y|\bx, \Phi) \Big] + 
\Big[ F_S(y|\bx, \Phi) - G \big[ F_S(y|\bx, \Phi) \big] \Big] dy \\
&= \underline{\int_{y \in \Ysc} 
\Big[ I(y>0) - F_S(y|\bx, \Phi) \Big] dy} + 
\int_{y \in \Ysc} 
\Big[ F_S(y|\bx, \Phi) - G \big[ F_S(y|\bx, \Phi) \big] \Big] dy
\end{align*}
Notice in the last line of above expression, the first integral (underlined) is the predictive mean with respect to the additive ensemble model $Y=\sum_{k=1}^K f_k(\bx)\mu_k + \delta(\bx) + \epsilon$. Therefore:
\begin{align}
E(y|\bx, G, \Phi) &= 
\sum_{k=1}^K f_k(\bx)\mu_k + 
\underbrace{\delta(\bx)}_{D_\delta(y|\bx)} + 
\underbrace{\int_{y \in \Ysc} 
\Big[ F_S(y|\bx, \Phi) - G \big[ F_S(y|\bx, \Phi) \big] \Big] dy}_{D_G(y|\bx)} \nonumber 
\\
&= \sum_{k=1}^K f_k(\bx)\mu_k + D_\delta(y|\bx) + D_G(y|\bx)
\label{eq:mean_decomp}
\end{align}
As shown, the predictive mean for full \gls{BNE} is composed of three parts: 1) the  predictive mean of the original ensemble $\sum_{k=1}^K f_k(\bx)\mu_k$, 2) the prediction error due to bias in prediction function $D_\delta(y|\bx)=\delta(\bx)$, and 3) the prediction error due to bias in distribution function $D_G(y|\bx)=\int \big[ F_S(y|\bx, \Phi) - G [ F_S(y|\bx, \Phi) ] \big] dy$. 

Consequently, we can assess the impact of model bias in distribution function and in distribution specification using $D_\delta$ and $D_G$:
\begin{align*}
D_\delta(y|\bx) &= \bdelta(\bx)
\\ 
D_G(y|\bx) &= \int \big[ F_S(y|\bx, \Phi) - G [ F_S(y|\bx, \Phi) ] \big] dy,
\end{align*}
and since both $\bdelta$ and $G$ are random variables, $D_G(y|\bx)$ and $D_\delta(y|\bx)$ are also random variables whose posterior distributions can be computed through the posterior distributions of $\bdelta$ and $G$.

\paragraph{Expression for Predictive Distribution's Other Properties}

We can generalize the above approach further to describe the impact of the distribution biases on other properties of the predictive distribution (e.g. predictive variance, skewness, multi-modality, etc). That is, given a summary statistic $s(y)$ that describes certain property of the predictive distribution, we can assess the impact of the distribution bias on such property as 
\begin{align}
D_{G} \big( s(y) | \bx \big) = \int \deriv{y} s(y) * \big[ \Phi(y|\bx, \mu) - G \big[ \Phi(y|\bx, \mu) \big] \big] dy,    
\label{eq:other_property}
\end{align}
and quantify the associated uncertainty using $P\big( D_{G} \big( s(y) | \bx \big) > 0 \big)$. For example, we can assess \textit{predictive variance} using the variance statistic $s(y) = (y-E(y))^2$, \textit{asymmetry} using the skewness statistic $s(y) = [(y-E(y))/SD(y)]^3$, and \textit{multi-modality} using the kurtosis statistic $s(y) = [(y-E(y))/SD(y)]^4$ \citep{bajgier_powers_1991, dagostino_tests_1973, yap_comparisons_2011}. In Section \ref{sec:exp} and \ref{sec:app_airpol}, we illustrate this method in experiments and apply it to detect a real-world ensemble system's systematic bias for air pollution prediction.

To derive (\ref{eq:other_property}), we again use the "Darth Vadar rule" (\ref{eq:darth}):
%we express a wide range of statistics $s(y)$ summarizing other properties of the model distribution $F(y|\bx, G, \Phi)$ in terms of decompositions similar to that for the predictive mean (\ref{eq:mean_decomp}). 
\begin{align*}
E(s(y)|\bx, G, \Phi)
&= \int_{y \in \Ysc} \deriv{y}s(y) \Big[ I(y>0) - F(y|\bx, G, \Phi) \Big] dy
\\
&= 
\underbrace{
\int_{y \in \Ysc} \deriv{y}s(y) \Big[ I(y>0) - F_S(y|\bx, \Phi) \Big] dy
}_{E\big( s(y)|\bx, \Phi \big)} 
+ 
\underbrace{
\int_{y \in \Ysc} \deriv{y}s(y)
\Big[ F_S(y|\bx, \Phi) - G \big[ F_S(y|\bx, \Phi) \big] \Big] dy}_{
D_G \big( s(y) | \bx \big)
}.
\\
&= E\big( s(y)|\bx, \Phi \big) + D_G \big( s(y) | \bx \big)
\end{align*}
where the first component $E\big( s(y)|\bx, \Phi \big)$ is the expected value of the summary statistics under the additive ensemble model $Y=\sum_{k=1}^K f_k(\bx)\mu_k + \delta(\bx) + \epsilon$, i.e. the \gls{BNE} model without $G$, and the second component $D_G \big( s(y) | \bx \big)$ is the change in $E(s(y)|\bx)$ due to model bias in distribution specification. 

Consequently, we can assess the impact of model bias in distribution function  on $E(s(y)|\bx)$ as:
\begin{align*}
D_G \big( s(y) | \bx \big) &= 
\int_{y \in \Ysc} \deriv{y}s(y)
\Big[ F_S(y|\bx, \Phi) - G \big[ F_S(y|\bx, \Phi) \big] \Big] dy
\end{align*}

\section{Uncertainty Decomposition with BNE}

\subsection{Structural Uncertainty Terms are Non-negative}
\label{sec:epi_comp_nonneg}
In this section, we show that the two structural uncertainty terms in the decomposition
\begin{align*}
\Isc \big((\omega, \delta, G), y \big| \bx \big) 
&=
    \underbrace{
    \Isc((\omega, \delta, G), y|\bx) - \Isc((\omega, \delta), y|\bx, G=I)
    }_{structural, G} + \\
&
    \underbrace{
    \Isc((\omega, \delta), y|\bx, G=I) - \Isc(\omega, y|\bx, \delta=0, G=I)
    }_{structural, \delta} + 
    \underbrace{
    \Isc(\omega, y|\bx, \delta=0, G=I)
    }_{parametric}
\end{align*}
are non-negative. We show this by showing a general result that for a parameter set $\Theta$  that can be partitioned into two groups $\Theta=\{\Theta_1, \Theta_2\}$, we always have:
\begin{align}
\Isc((\Theta_1, \Theta_2), y|\bx) - \Isc(\Theta_1, y|\bx, \Theta_2=\theta_2) \geq 0    
\label{eq:nonneg_general}
\end{align}
If we can show (\ref{eq:nonneg_general}), then we have shown the two structural uncertainty terms are non-negative by taking $\Theta_1 = \omega$ and $\Theta_2 = (\delta, G)$ for structural uncertainty in $\delta$, and $\Theta_1 = (\omega, \delta)$ and $\Theta_2 = G$ for structural uncertainty in $G$.

We now show (\ref{eq:nonneg_general}) is true. Show this by showing below two inequalities:
\begin{align}
    \Isc((\Theta_1, \Theta_2), y|\bx) &\geq \Isc((\Theta_1, \Theta_2=\theta_2), y|\bx)
    \label{eq:nonneg_first_ineq}
    \\
    \Isc((\Theta_1, \Theta_2=\theta_2), y|\bx) &\geq \Isc(\Theta_1, y|\bx, \Theta_2=\theta_2)
    \label{eq:nonneg_second_ineq}
\end{align}

First show (\ref{eq:nonneg_first_ineq}), notice that:
\begin{align*}
    \Isc((\Theta_1, \Theta_2), y|\bx)
    &= 
    \int f(\Theta_1, \Theta_2, y|\bx) 
    log \frac{f(\Theta_1, \Theta_2, y|\bx)}
    {f(\Theta_1, \Theta_2|\bx) f(y|\bx)} d\Theta_1 dy\\
    &= 
    \int f(\Theta_1, \Theta_2|\bx) * f(y|\Theta_1, \Theta_2, \bx)
    log \frac{f(y|\Theta_1, \Theta_2, \bx)}
    {f(y|\bx)} d\Theta_1 dy\\
    &= 
    \int f(\Theta_1, \Theta_2|\bx) * 
    KL \Big[ f(y|\Theta_1, \Theta_2, \bx) || f(y|\bx) \Big] d(\Theta_1, \Theta_2)
    \\
    &\geq 
    \int f(\Theta_1, \Theta_2|\bx) * 
    KL \Big[ f(y|\Theta_1, \Theta_2, \bx) || f(y|\bx) \Big] d(\Theta_1, \Theta_2=\theta_2)
    \\
    &= 
    \int f(\Theta_1, \Theta_2=\theta_2, y|\bx) 
    log \frac{f(\Theta_1, \Theta_2=\theta_2, y|\bx)}
    {f(\Theta_1, \Theta_2=\theta_2|\bx) f(y|\bx)} d\Theta_1 dy
    \\
    &=
    \Isc((\Theta_1, \Theta_2=\theta_2), y|\bx)
\end{align*}
where the first inequality in above expression follows since the KL term is always non-negative. Now show  (\ref{eq:nonneg_second_ineq}):
\begin{align*}
    \Isc((\Theta_1, \Theta_2=\theta_2), y|\bx) 
    &= 
    \int f(\Theta_1, \Theta_2=\theta_2, y|\bx) 
    log \frac{f(\Theta_1, \Theta_2=\theta_2, y|\bx)}
    {f(\Theta_1, \Theta_2=\theta_2|\bx) f(y|\bx)} d\Theta_1 dy
    \\
    &= 
    \int f(\Theta_1, \Theta_2=\theta_2, y|\bx) 
    \Big[
    log \frac{f(\Theta_2=\theta_2, y|\bx)}
    {f(\Theta_2=\theta_2|\bx) f(y|\bx)} + 
    log \frac{f(\Theta_1, y|\bx, \Theta_2=\theta_2)}
    {f(\Theta_1|\bx, \Theta_2=\theta_2) f(y|\bx, \Theta_2=\theta_2)}    
    \Big]
    d\Theta_1 dy
    \\
    &=
    KL\Big[f(\Theta_2=\theta_2, y|\bx) || f(\Theta_2=\theta_2|\bx) f(y|\bx) \Big] + 
    \Isc(\Theta_1, y|\bx, \Theta_2=\theta_2)
    \\
    & \geq \Isc(\Theta_1, y|\bx, \Theta_2=\theta_2)
    ,
\end{align*}
and the inequality follows since the KL divergence is always non-negative. 

Finally, by combining (\ref{eq:nonneg_first_ineq}) and (\ref{eq:nonneg_second_ineq}), we have shown (\ref{eq:nonneg_general}).

\clearpage
\section{Experiments}
%\subsection{1D Experiments}
\label{sec:app_exp_1d}

\subsection{Data Generation Mechanism and Computation Environment}

We sample $x$ from a mixture of Gaussians $\{N(-4, 0.4), N(0, 1), N(4, 0.4) \}$, and sample $y$ from $y = 7*sin(x) + 3 *cos(\frac{x}{2})\epsilon$ with $\epsilon \sim Weibull(\alpha, \beta=1)$. We set $\alpha=3*exp(-|x|)$ so the noise distribution is highly skewed and heavy-tailed at the margin of input space $x \in \Xsc$ but is symmetric (i.e. low skewness) in the middle. All computation is done on a Intel Core i7-6700HQ machine with Nvidia GeForce GTX 1070 GPU and 16 Gb RAM. Implementation is done in TensorFlow Probability under Ubuntu 14.04 LTS \citep{dillon_tensorflow_2017}. 

\subsection{Visualization of Base Models}

For base models $\{f_k\}_{k=1}^K$, we pre-train 3 kernel ridge regression models on half of the data points, using periodic and \gls{RBF} kernels as their kernel families (see Figure \ref{fig:base_model_hetero_app} for an example). We then train the ensemble model using the remaining half of the data points.

\begin{figure*}[ht]
    \centering
    \begin{subfigure}{0.45\textwidth}
        \includegraphics[width=\textwidth]{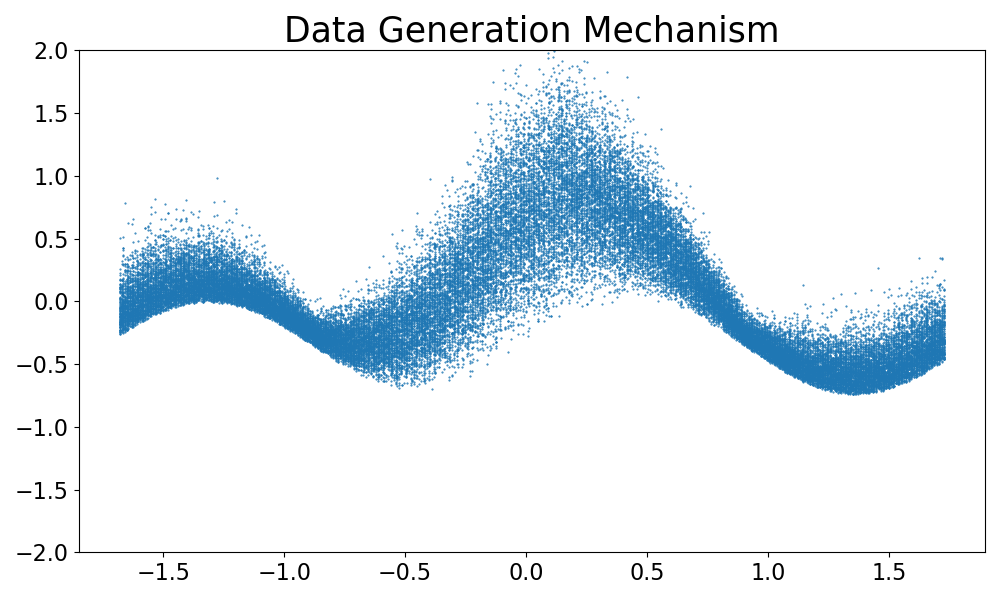}
        \caption{}        
        \label{fig:data_hetero_app}        
    \end{subfigure}
    \begin{subfigure}{0.45\textwidth}
        \includegraphics[width=\textwidth, height=4cm]{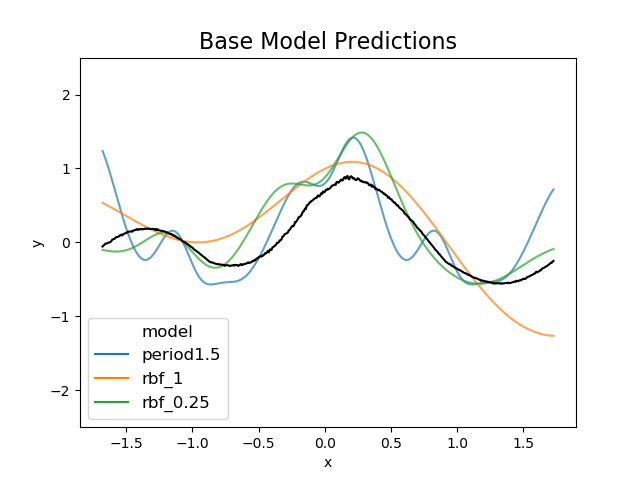}
        \caption{}        
        \label{fig:base_model_hetero_app}        
    \end{subfigure}     
    \caption{
    \textbf{Left}: data generation mechanism; 
    \textbf{Right}: base model predictions (fitted with 50 training data points). 
}
\label{fig:exp_1d_hetero}
\end{figure*}

\subsection{Further Description of Experiment Results}

\paragraph{Uncertainty-aware Model Bias Detection} We quantify the impact of the original ensemble's model biases on model's predictive distribution in Figure \ref{fig:impact_mean_misspec_hetero} and \ref{fig:impact_random_misspec_hetero}. Recall as discussed in Section \ref{sec:impact_unc}, such impact are quantified by the random quantity $D_{\delta}$ and $D_{G}$, respectively, and model's posterior confidence in such impact are described by the probabilities $P\big( D_{\delta} > 0 \big)$ and $P\big(D_{G} > 0 \big)$. Figure \ref{fig:impact_mean_misspec_hetero} shows model's posterior confidence in original ensemble's predictive bias due to misspecification in prediction function (color indicates the direction of the bias). As shown, the high-confidence regions in \ref{fig:impact_mean_misspec_hetero} precisely reflected regions in  \ref{fig:unc_decomp_mean_hetero} where model bias exists and data is available. Specifically, the confidence is high if the model bias is severe or there are enough data to justify the existence of bias, and is low otherwise. Figure \ref{fig:impact_random_misspec_hetero} shows model's posterior confidence in Bayesian additive ensemble's bias in predictive mean (upper plot) and variance (lower plot) due to misspecification in the distribution function. As shown, the high-confidence regions in the upper plot of Figure \ref{fig:impact_random_misspec_hetero} precisely captured  regions where biases in the predictive mean exist (see Figure \ref{fig:unc_decomp_resid_hetero}). Specifically, notice that in regions where the data is sufficient (e.g. $x \in [1.0, 1.5]$), the posterior confidence is able to identify biases in predictive mean even if their magnitude is small. Finally, in the lower plot of Figure  \ref{fig:impact_random_misspec_hetero}, model's posterior confidence in variance bias accurately captured regions where the additive ensemble model fail to account for the decreased variance in data's empirical distribution on the left and right margin of the feature space $x \in \Xsc$.

\section{Application}
\label{sec:app_application}

\subsection{Background}
To assess exposure in air pollution health studies, many research groups are developing distinct spatial models (exposure models) to predict ambient air pollution concentrations even in areas where air pollution monitors are sparse. 
%It is becoming a standard practice in the field to develop ensemble systems aggregating different exposure models to improve prediction accuracy. However, 
These different models have different inputs (including remote sensing, chemical transport models, and land use variables) and employ different algorithms (e.g., generalized additive models, random forests and neural networks). As a result, the model predictions from base models differ across space; if these were to be integrated in an ensemble model, thus, the variability among the base model predictions would drive the predictive uncertainty (e.g., see Figure \ref{fig:app_ensemble_base}). %Furthermore, although each of these base models is trained to maximize the out-of-sample accuracy in predicting daily air pollution concentrations, recent studies have found that the prediction performance deteriorates noticeably when averaging these daily predictions to predict monthly or annual average concentrations, suggesting the existence of model bias in predicting long-term air pollution concentrations. 
%\mak{i thought we had said you wouldn't include this text (since no published studies actually exist); i commented it out}
Consequently, for the purpose of model validation and refinement, it is important to identify the spatial regions where model bias exists, and how disagreement across candidate models may significantly impact the ensemble's predictive uncertainty.

\begin{figure}[ht]
    \centering
    \begin{subfigure}{0.32\textwidth}
        \includegraphics[width=\textwidth]{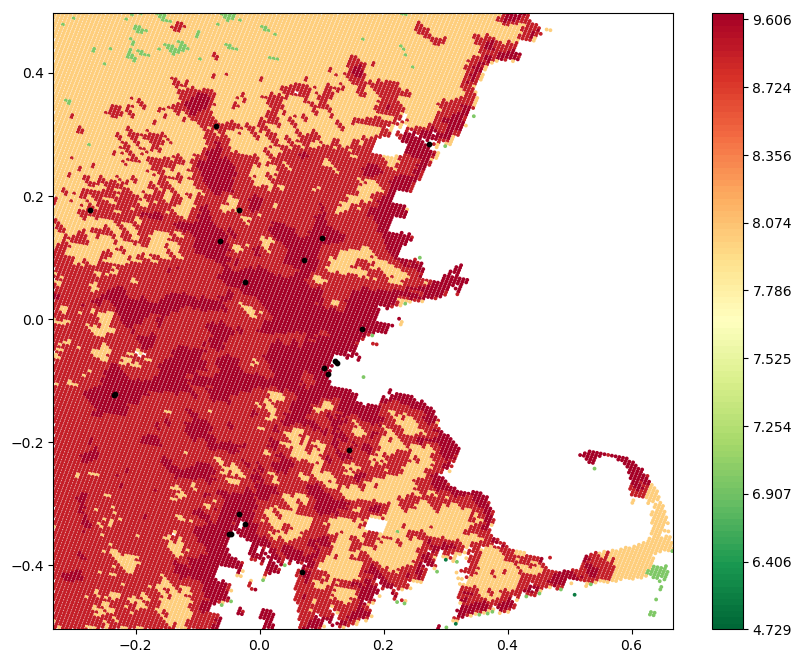}
    \end{subfigure}
    \begin{subfigure}{0.32\textwidth}
        \includegraphics[width=\textwidth]{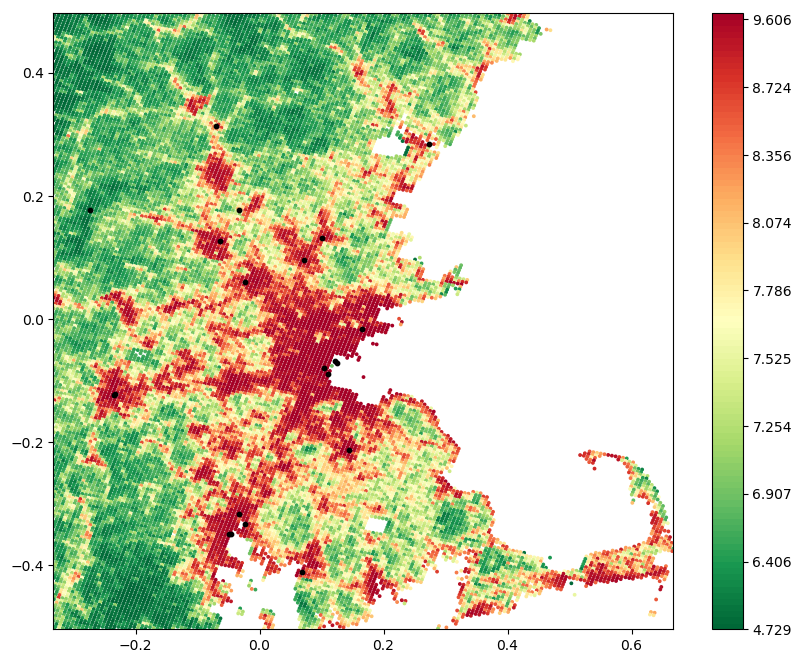}
    \end{subfigure}
    \begin{subfigure}{0.32\textwidth}
        \includegraphics[width=\textwidth]{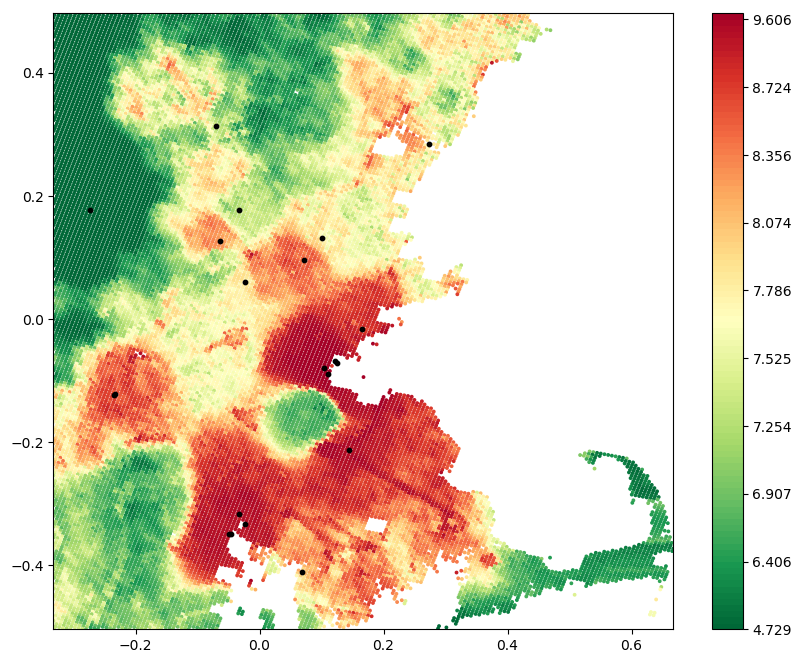}
    \end{subfigure}      
    \caption{Visualization of 2011 $PM_{2.5}$ predictions from different base models in Eastern Massachussets, USA. \textbf{Left} \citep{donkelaar_global_2016}, \textbf{Middle}:  \citep{kloog_new_2014}, \textbf{Right}:  \citep{di_hybrid_2016}  }
   \label{fig:app_ensemble_base}
\end{figure}

\subsection{Results}
\begin{table}[!ht]
\centering
\scalebox{1.0}{
\begin{tabular}{ccccc}
\hline%\hline
Model & \textbf{BNE} & \textbf{BME} & \textbf{BAE} & \textbf{stack} \\
\hline
loo RMSE & $0.762 \pm 0.09$ & $0.833 \pm 0.07$ & $1.077 \pm 0.13$ & $1.472 \pm 0.15$ 
\\
\hline%\hline
\end{tabular}
}
\caption{Mean and Standard Deviation for leave-one-out cross-validation RMSE \\ in the 2011 PM$_{2.5}$ ensemble prediction.}
\label{tb:app_comp}
\end{table}

\begin{figure}[ht]
\centering
    \includegraphics[width=.48\columnwidth]{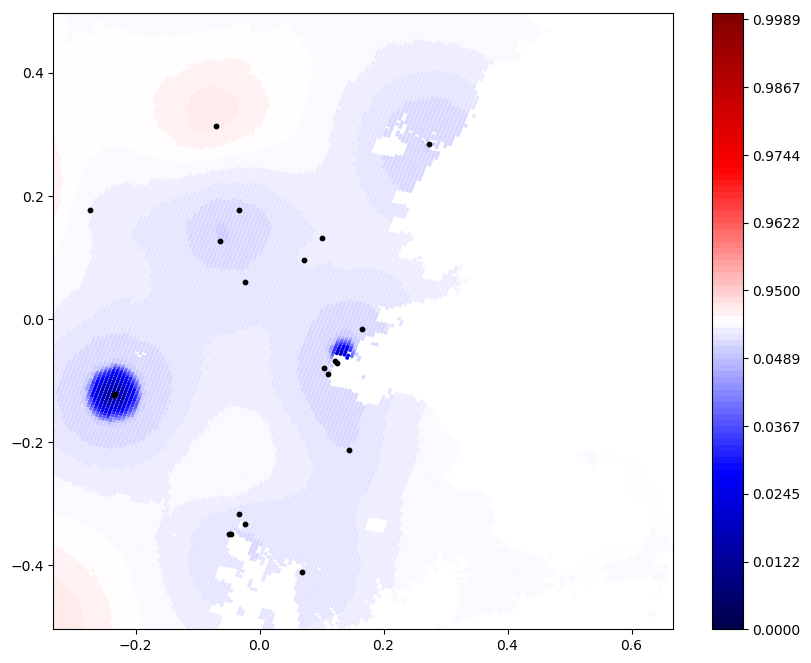}
    \caption{Posterior confidence in original model's prediction bias, i.e. $P(D_\delta(y|\bx)>0)$. Blue/Red color indicates evidence of over-/under-estimation}
    \label{fig:app_bias}
\end{figure}

%\begin{wrapfigure}[21]{r}{0.38\textwidth}
%    \includegraphics[width=.48\columnwidth]{"./plots/app/impact_resid"}
%    \caption{Posterior confidence in original model's prediction bias, i.e. $P(D_\delta(y|\bx)>0)$. Blue/Red color indicates evidence of over-/under-estimation}
%    \label{fig:app_bias}
%\end{wrapfigure}
